# Supplementary material for: A Dataset-Dispersion Perspective on Reconstruction Versus Recognition in Single-View 3D Reconstruction Networks
Source: arXiv:2111.15158 source file (2021-11-30)
Supplement: Supplementary file 2 [file 1-supplementary.tex]

\section{Synthetic Data Generation}\label{sec:conclusion}

We use the software Blender to generate base shapes in a mesh format. Then, we use the Shrinkwrap modifier in ``Nearest Vertex'' mode to define the shape morphing between the two base shapes and control the interpolation progress by the Blender Shape Keys panel. After creating the mesh dataset, we render training images and sample point cloud from mesh.

\begin{figure*}[!thb] 
  \captionsetup[subfigure]{labelformat=empty}
  \begin{centering}
  \begin{subfigure}[b]{0.124\linewidth}
       \includegraphics[width=\linewidth]{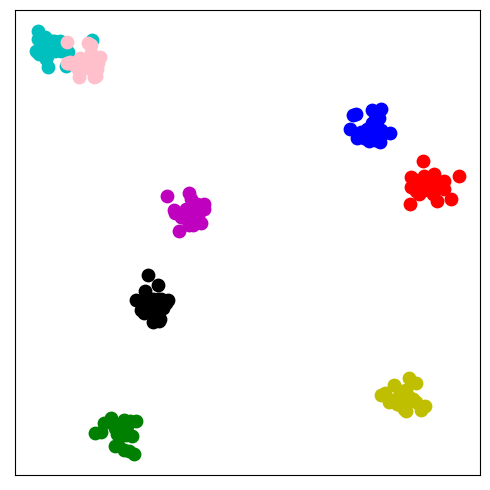}
       \caption{\small cluster std=1}
   \end{subfigure}\hspace*{-0.4em}
  \begin{subfigure}[b]{0.124\linewidth}
       \includegraphics[width=\linewidth]{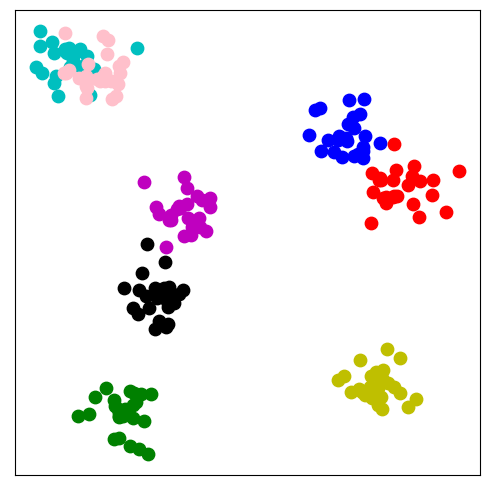}
       \caption{\small cluster std=2}
   \end{subfigure}\hspace*{-0.4em}
  \begin{subfigure}[b]{0.124\linewidth}
       \includegraphics[width=\linewidth]{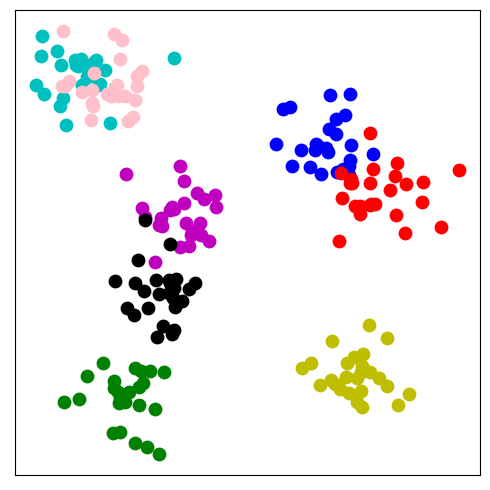}
       \caption{\small cluster std=3}
   \end{subfigure}\hspace*{-0.4em}
  \begin{subfigure}[b]{0.124\linewidth}
       \includegraphics[width=\linewidth]{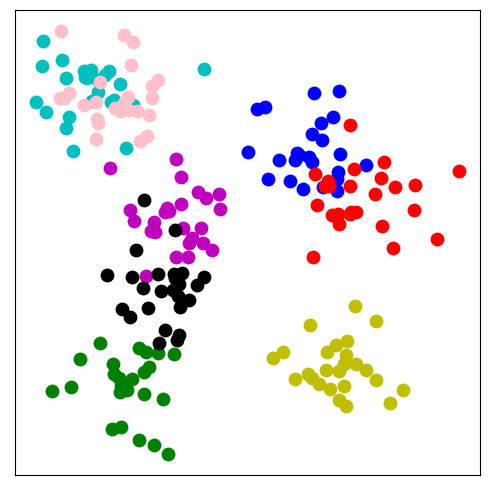}
       \caption{\small cluster std=4}
   \end{subfigure}\hspace*{-0.4em}
  \begin{subfigure}[b]{0.124\linewidth}
       \includegraphics[width=\linewidth]{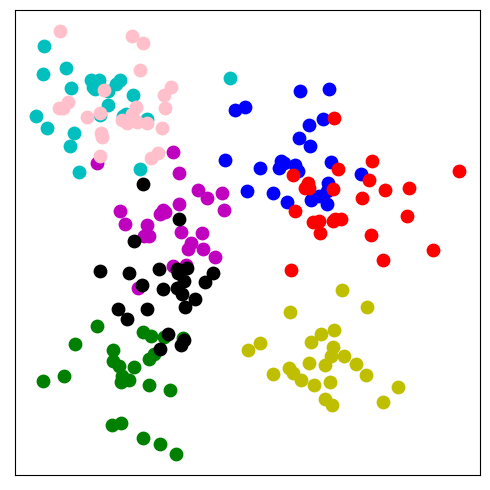}
       \caption{\small cluster std=5}
   \end{subfigure}\hspace*{-0.4em}
  \begin{subfigure}[b]{0.124\linewidth}
       \includegraphics[width=\linewidth]{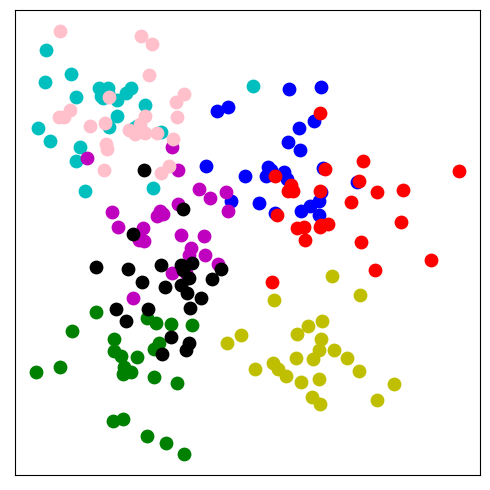}
       \caption{\small cluster std=6}
   \end{subfigure}\hspace*{-0.4em}
  \begin{subfigure}[b]{0.124\linewidth}
       \includegraphics[width=\linewidth]{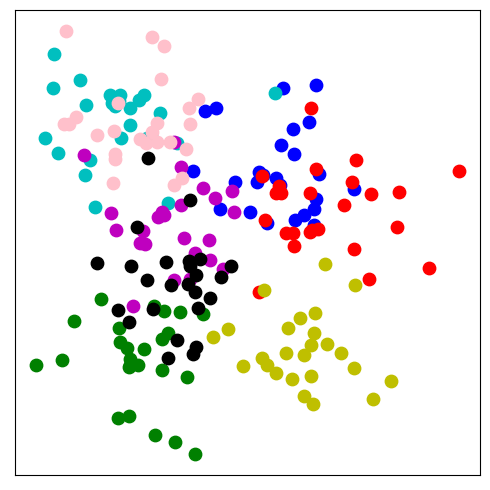}
       \caption{\small cluster std=7}
   \end{subfigure}\hspace*{-0.4em}
  \begin{subfigure}[b]{0.124\linewidth}
       \includegraphics[width=\linewidth]{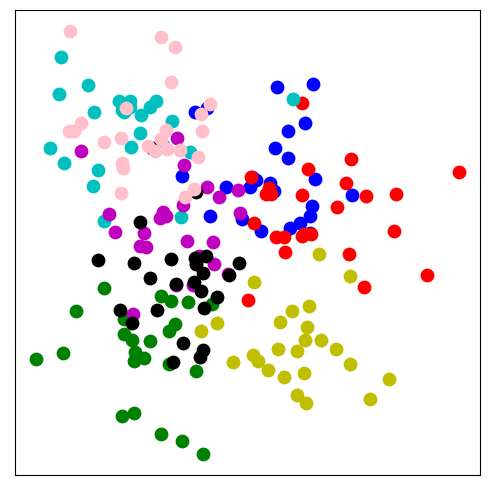}
       \caption{\small cluster std=8}
   \end{subfigure}
   \end{centering}
   \caption{\small Visualization of toy datasets created for demonstrating dispersion score. Data points with the same color means the data is belong to a common cluster. From left to right, datasets become more dispersed as the standard deviation of the clusters increase by 1}
   \label{fig:2d-toy-datasets}
\end{figure*}

\begin{figure}[!thb]
  \centering
  \includegraphics[width=.95\columnwidth]{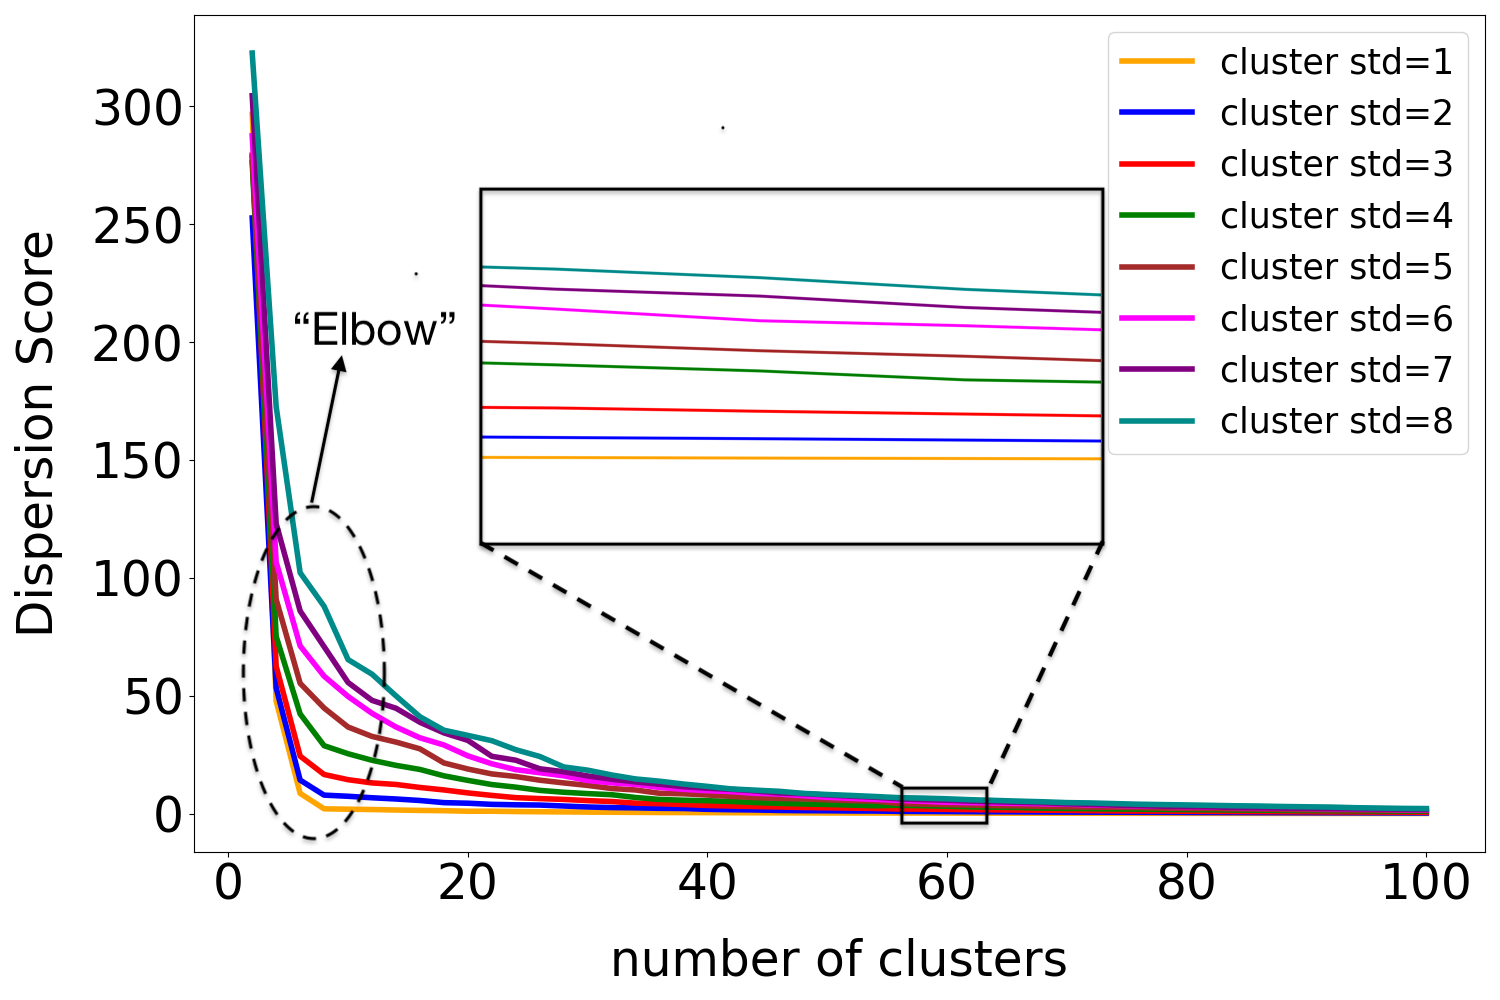}
  \caption{\small Dispersion score with varying hyperparameter "number of clusters" in evaluation of 2D toy datasets. The metric, dispersion score is effective to measure how dispersed the dataset is as more dispersed dataset shows larger dispersion score. ``Elbow'' is the point of inflection on the curve. As number of clusters increase to larger than the value of ``Elbow'', the dispersion score become insensitive to hyperparameter.}
  \label{fig:num-clusters-search}
\end{figure}

Regarding how to choose the hyperparameter, the number of clusters, we suggest to do a parameter sweeping, and choose the value of cluster number larger than the ``Elbow'' of dispersion score curve as parameter for the metric. ``Elbow'' is the point of inflection on the curve of dispersion score with varying number of clusters. We further use examples to demonstrate how to choose the hyperparameter and the effectiveness of the metric. See Figure \ref{fig:2d-toy-datasets}, We build a group of eight 2D toy datasets. For each dataset, we generate 200 2D points which forms 8 clusters. We change clustering degree by increasing the cluster standard deviation (std\ by 1, so the eight datasets become increasing dispersed. We evaluate the dispersion score of eight toy datasets with varying number of clusters from 2 to 100 with step 2. The distance function is squared euclidean distance. In Figure \ref{fig:num-clusters-search}, we show the position of ``Elbow'' on the curve, and the dispersion score become insensitive to hyperparameter when the hyperparameter increase to larger than the value of "Elbow". Therefore, we suggest evaluating the dispersion score at number of clusters equal to the value of ``Elbow'' and larger. Besides, in figure \ref{fig:num-clusters-search}, since dataset with larger cluster std is more dispersed, we can see the dispersion score of more dispersed dataset is larger. Thus, we further demonstrate  dispersion score is effective to measure the how dispersed the data is.

\begin{figure}
  \centering
  \begin{subfigure}[b]{0.49\columnwidth}
       \centering
       \includegraphics[width=\linewidth]{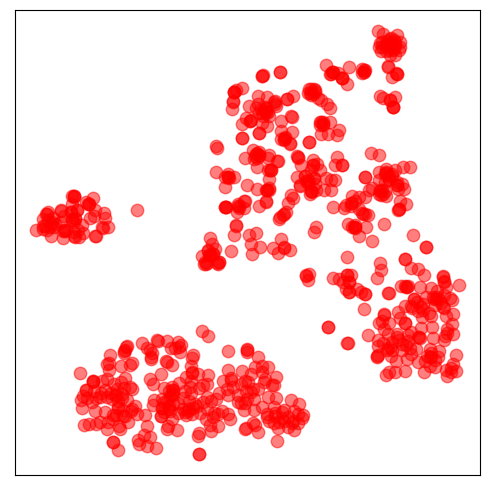}
       \caption{}
   \end{subfigure}
   \begin{subfigure}[b]{0.49\columnwidth}
        \centering
        \includegraphics[width=\linewidth]{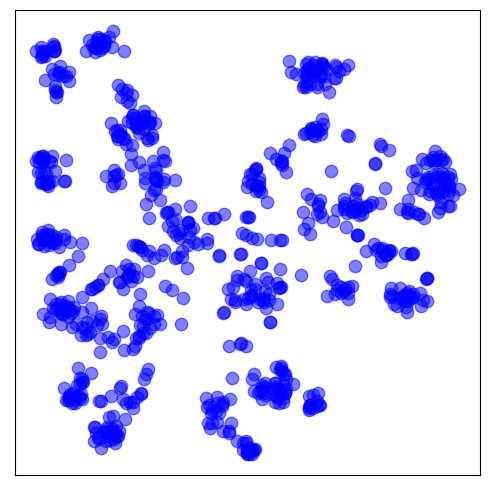}
        \caption{}
   \end{subfigure}
   \begin{subfigure}[b]{0.84\columnwidth}
        \centering
        \includegraphics[width=\linewidth]{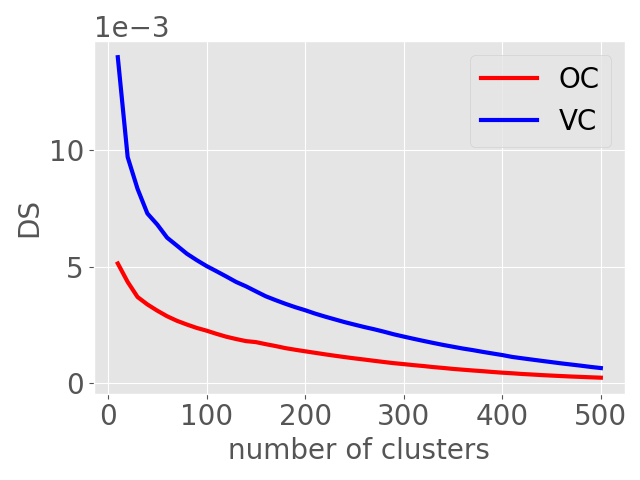}
        \caption{}
   \end{subfigure}
   \caption{Shape set in object-centered is more clustered while viewer-centered coordinate is more dispersed. (a) t-SNE of distance matrix of object-centered shapes in ShapeNet airplane. (b) t-SNE of distance matrix of viewer-centered shapes in ShapeNet class airplane. (c) The dispersion score of viewer-centered shape set is larger than that of object-centered with varying number of clusters.}
   \label{fig:oc-vc-dispersion-demo}
\end{figure}

To demonstrate the difference of dispersion degree between two coordinate representation, in Figure \ref{fig:oc-vc-dispersion-demo} we show the shape set of airplane class in ShapeNet \cite{chang2015shapenet}. We show that shape set in object-centered is more clustered than that in viewer-centered by two methods,  t-SNE~\cite{10.5555/2968618.2968725} and dispersion score proposed in \ref{sec:metric_on_dataset}. Note that the total instance amount of airplane class is 809, the parameter sweeping on number of clusters is from 10 to 500 with step size 10. We use Chamfer Distance as distance function in distance matrix computation.

We investigate if more training samples can guide NN to perform more reconstruction in SVR. Note that the ``more training samples'' is obtained by using more rendering images that have been given in ShapeNetCore~\cite{choy20163d}, the shape topology and amount of 3D models remain unchanged. The conventional setup in \cite{choy20163d, groueix2018papier} is to use one view of image among 24 views per model for each epoch, but in this experiment, for each epoch, we use more views per model range from 1 to 18. Since we also use VC coordinate, as mentioned in \ref{sec:definition-coordinate}, shape is rotated based on input viewpoint of rendering image. Thus, using more views per model is equivalent to using more training images and more training shapes augmented by 3D rotation. The amount of training data is multiplied by the number of views per model. The results are reported in Figure \ref{fig:nviews-search}. First, Figure \ref{fig:nviews-inertia} shows that there is certain gap between improved output DS (0.720) of NN trained on 18$\times$ more samples and GT (0.010), and the rising trend has been converged. It indicates that it is challenging to further improve NN to perform reconstruction based on current published dataset and simple data augmentation like rotation. Stronger data augmentation that can augment topology of shapes are needed in future search. Second, Figure \ref{fig:nviews-chamfer} shows that the performance trend given by output DS is consistent with that of CD and F-score, further verifying the effectiveness of output DS as a metric to evaluate model performance and guide data augmentation in SVR.

\begin{figure}[h!]
    \centering
    \begin{subfigure}[b]{0.49\columnwidth}
        \includegraphics[width=\linewidth]{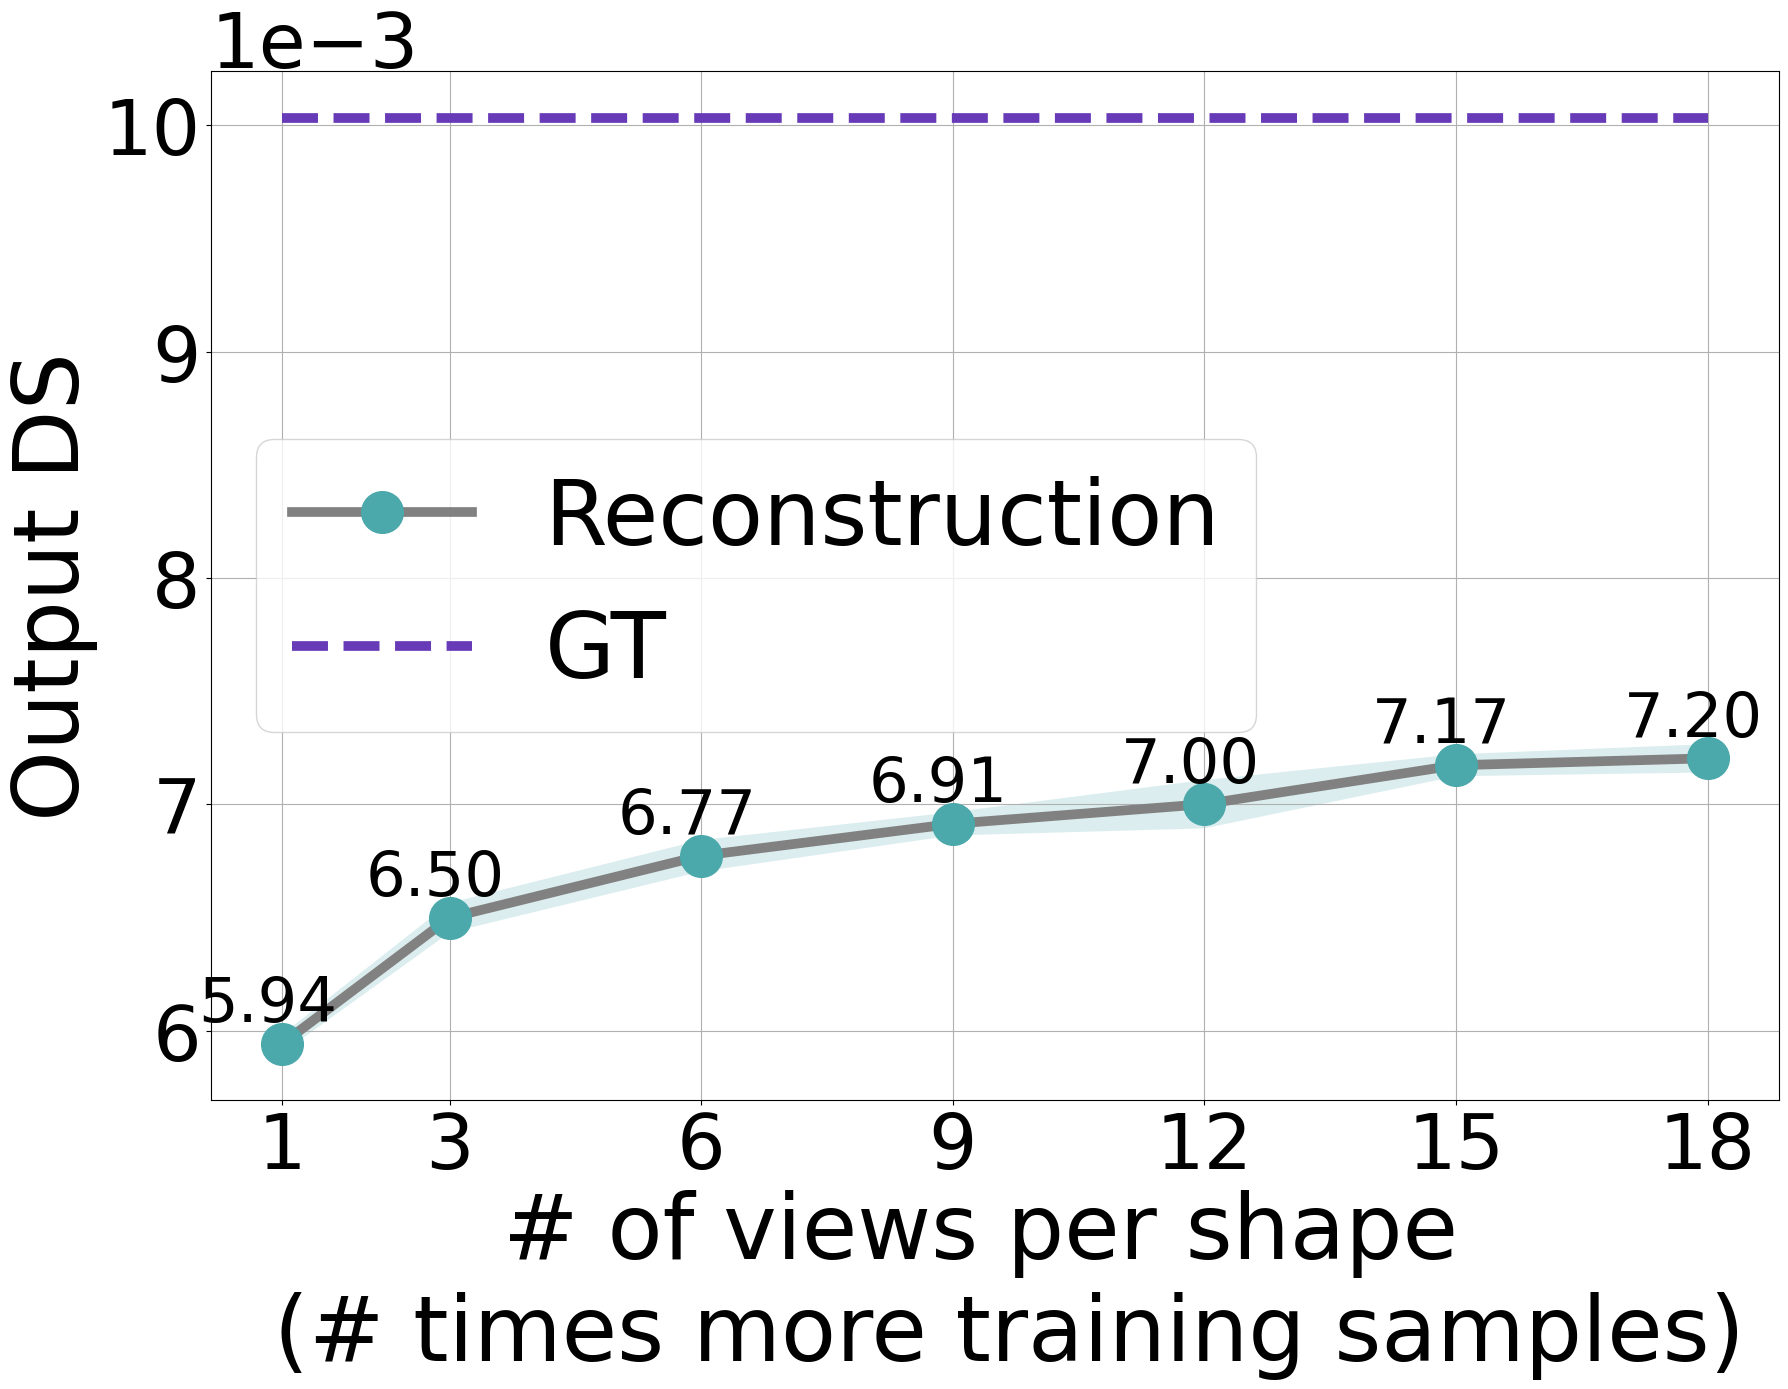}
    \caption{\small }\centering
    \label{fig:nviews-inertia-supp}
    \end{subfigure}
    \begin{subfigure}[b]{0.49\columnwidth}
        \includegraphics[width=\linewidth]{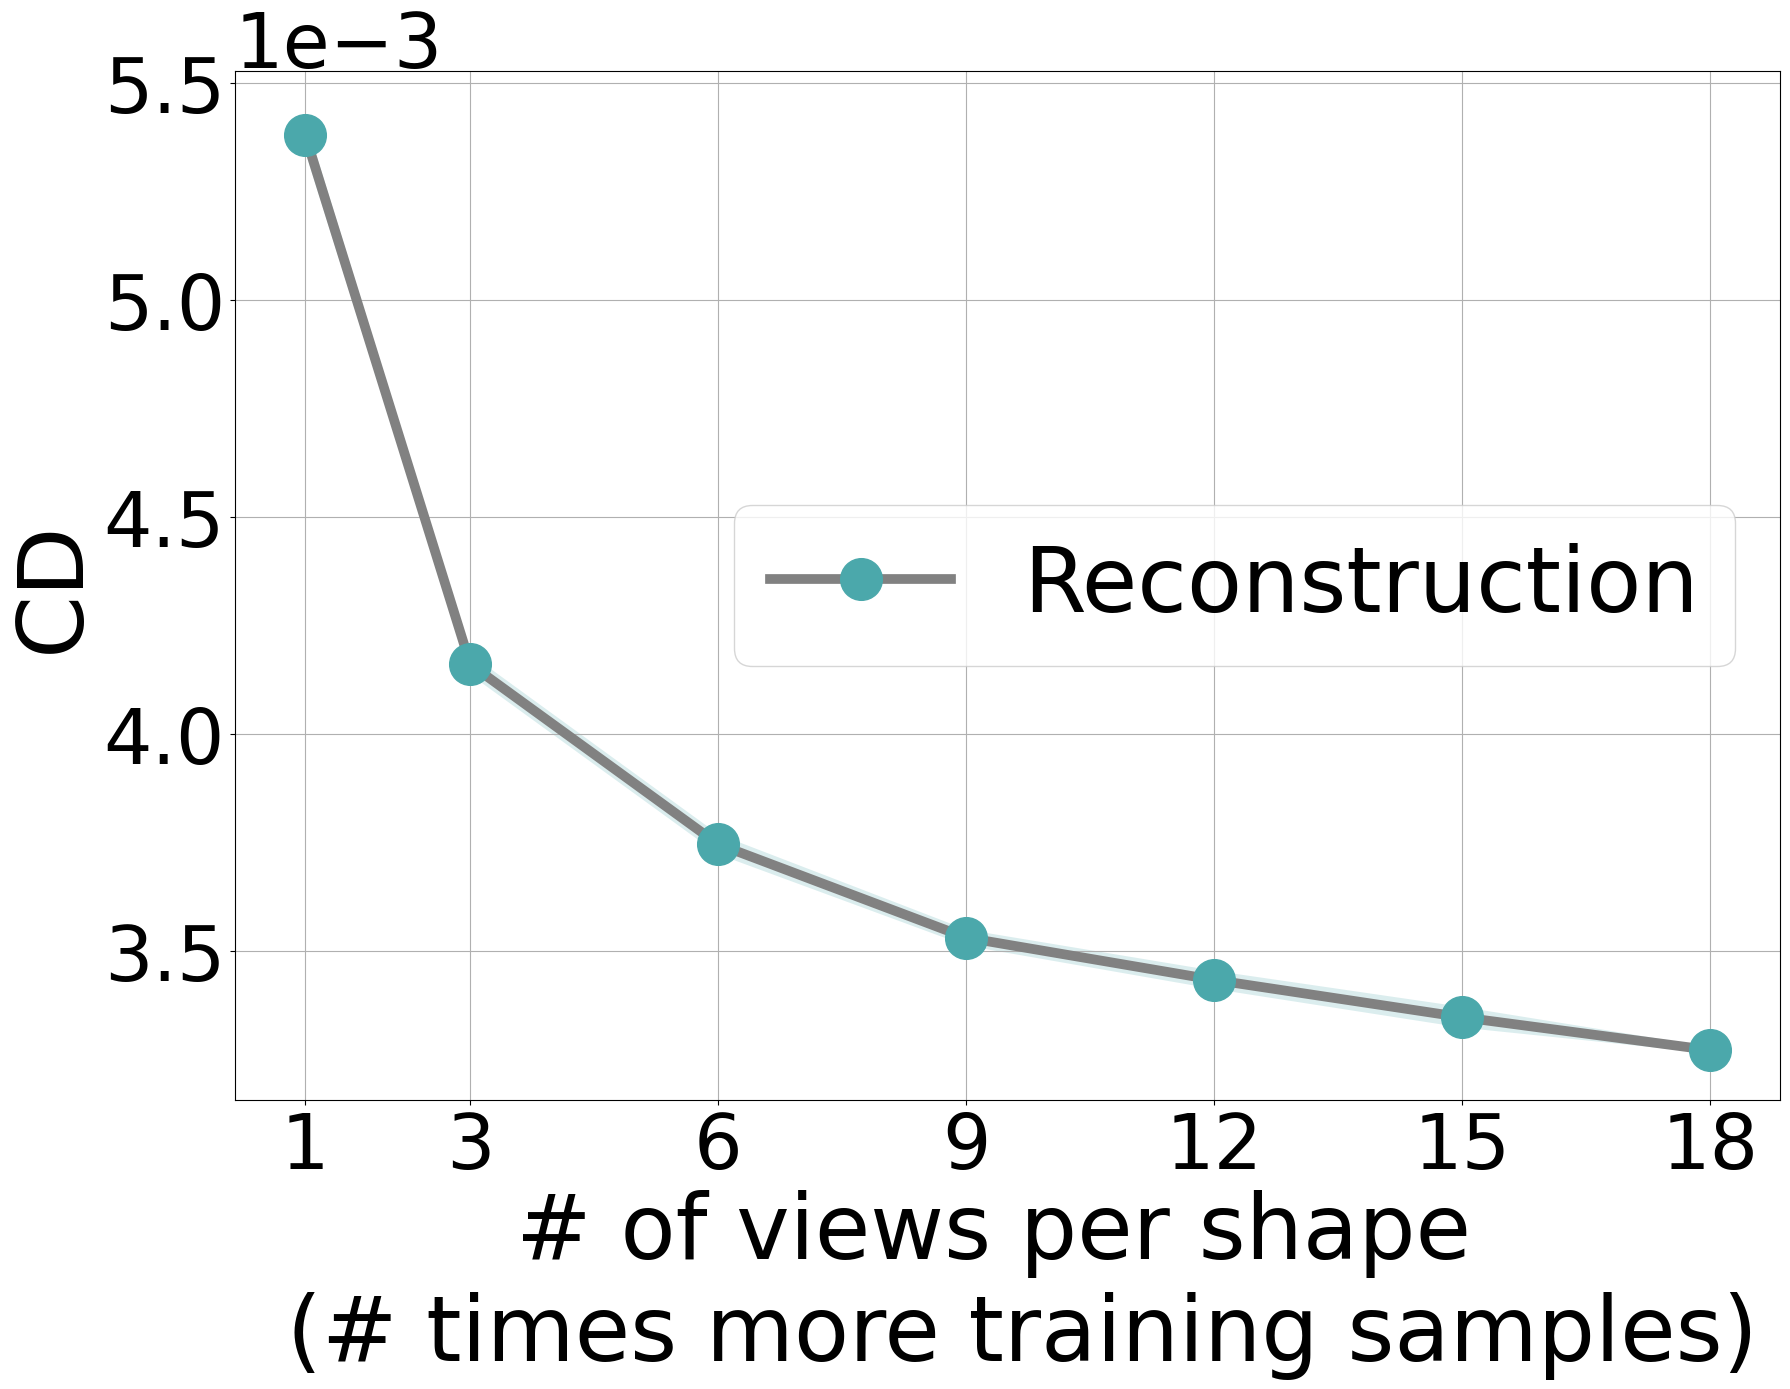}
    \caption{}\centering
    \label{fig:nviews-chamfer-supp}
    \end{subfigure}
   \caption{\small Evaluation of models trained on more training samples in VC coordinate. Using more number of views per model in VC is equal to multiplying the amount of training samples. The capability of NN to perform reconstruction is limited even using 18$\times$ more training data. (a) Output DS($\uparrow$) (b) F-score($\uparrow$) and CD($\downarrow$)} 
   
   \label{fig:nviews-search-supp}
\end{figure}
